# Supplementary material for: AlphaPIG: The Nicest Way to Prolong Interactive Gestures in Extended Reality
Source: arXiv:2503.01011 source file (2025-03-02)
Supplement: Supplementary file 1 [file 1_part_one.tex]

\pagebreak
\section{Appendix}

\begin{figure}
    \centering
    \includegraphics[width=0.45\linewidth]{figures/Q1_conditions.png}
    \includegraphics[width=0.45\linewidth]{figures/Q2_conditions.png}
    \\
    \includegraphics[width=0.45\linewidth]{figures/Q3_conditions.png}
    \includegraphics[width=0.45\linewidth]{figures/Q4_conditions.png}
    \caption{%\textbf{Left:} 
    Distribution of participants' answers to questions Q1-Q4 on a scale from -3 to 3, for different study conditions.
    Conditions are shown on the y-axis and percentages of participants that gave a particular answer on the x-axis.
    % \textbf{Right:} Answer scores averaged over all study participants, for different levels of \textit{Timing} (x-axis) and \textit{DecayRate} (y-axis), and for questions Q1-Q4.
    }
    \label{fig:Questionnaire_comparison_detailed}
\end{figure}
